# Supplementary material for: MLRS-PDS: A Meta-learning recommendation of dynamic ensemble selection pipelines
Source: arXiv:2407.07528 source file (2024-07-10)
Supplement: Supplementary file 1 [file supplementary_material.tex]

\section{Meta-features}

Below is a brief description of each category:

\begin{itemize}
    \item \textbf{Statistical}: There are standard statistical measures to describe the numerical properties of data distribution (\citerefs{brazdil2008metalearning}). This category for extracting statistical meta-features from datasets covers a range of statistical computations, including computing correlations, covariances, median, minimum, and maximum values, and various other statistical measures for each attribute. 
    
    \item \textbf{Information-theoretic}: It encompasses a diverse set of measures used to analyze datasets' characteristics. They include the assessment of class label and attribute entropy, the quantification of relationships between variables, the evaluation of signal-to-noise ratios, and the estimation of effective attributes (\citerefs{brazdil2008metalearning}).
    
    \item \textbf{Model-based}: meta-features that are designed to capture characteristics of machine learning models, specifically Decision Tree (DT) models, induced from a dataset. These meta-features encompass specific properties, including depth, shape, and size, which can be indicative of the complexity and structure of the dataset. (\citerefs{pavel2002decision}).
    
    \item \textbf{Landmarking}: Performance of simple and efficient learning algorithms such as DEcision trees (DT) and K Nearest neighbors (KNN). The meta-features, $m_{f}$, collected in this category include relative and subsampling performances (\citerefs{reif2014automatic, smith2009cross, rivolli2018characterizing}, soares2001sampling).
    
    \item \textbf{Clustering-based}: This meta-feature collects information regarding both correlation and dissimilarity. The Correlation Measure quantifies the statistical relationships between pairs of instances in the dataset. The stronger similarity in attribute behaviors among instances results in a higher correlation. The Dissimilarity Measure is based on the Euclidean distance between instances, representing the distance between data points in the dataset (\citerefs{pimentel2019new}).
    
    \item \textbf{Concept}: Estimate the variability of class labels among examples and the example's density. 
    (\citerefs{rivolli2018characterizing}). Methods for extracting meta-features related to the Concept group from datasets cover computations such as cohesiveness, concept variation, improved concept variation, and weighted distance between examples of the same classes as well as different classes. Hence, they are measures to define whether a feature space is highly irregular (several small groups of samples belonging to the same class) or more uniform in which large regions of samples share the same class labels.
    
    \item \textbf{Itemset}: Compute the correlation between binary attributes (\citerefs{song2012automatic}).
    
    \item \textbf{Complexity}: Estimate the difficulty in separating the data points into their expected classes (\citerefs{lorena2019complex}). The extraction of meta-features related to dataset complexity involves various methods, covering computations such as entropy, imbalance ratio, clustering coefficient, network density, Fisher's discriminant ratios, hub scores, and a range of other complexity measures.
\end{itemize}

The list describing all meta-features considered in this work is presented in the Tables below:

\begin{table}[H]
\centering
\begin{minipage}{0.9\linewidth}
\caption{Meta-features present in the meta-dataset}
\label{mfff}
\scalebox{0.7}{
\begin{tabular}{|l|l|l|l|}
\hline
  & Meta feature & Group & Description \\
\hline

1  &  attr\_to\_inst & general & Compute the ratio between the number of attributes. \\

2  &  cat\_to\_num & general & Compute the ratio between the number of categoric and numeric features. \\
 
3  &  freq\_class & general & Compute the relative frequency of each distinct class. \\
% 3  &  freq\_class\_sd & general & Compute the standard deviation of the relative frequency of each distinct class. \\
 
4  &  inst\_to\_attr & general & Compute the ratio between the number of instances and attributes. \\
 
5  &  nr\_attr & general & Compute the total number of attributes. \\
 
6  &  nr\_bin & general & Compute the number of binary attributes. \\
 
7  &  nr\_cat & general & Compute the number of categorical attributes. \\
 
8  &  nr\_class & general & Compute the number of distinct classes. \\
 
9  &  nr\_inst & general & Compute the number of instances (rows) in the dataset. \\
 
10  &  nr\_num & general & Compute the number of numeric features. \\
 
11  &  num\_to\_cat & general & Compute the number of numerical and categorical features. \\
 
12  &  precompute\_general\_class & general & Precompute distinct classes and its frequencies from y. \\
 % nadasht 12
13  &  can\_cor & Statistical & Compute the canonical correlations of data. \\

% 13  &  can\_cor\_sd & Statistical & Compute the standard deviation of the canonical correlations of data. \\
 
14  &  cor & Statistical & Compute the absolute value of the correlation of distinct dataset column pairs. \\

% 14  &  cor\_sd & Statistical & Compute the standard deviation of the absolute value of the correlation of distinct dataset column pairs. \\
 
15  &  cov & Statistical & Compute the absolute value of the covariance of distinct dataset attribute pairs. \\
 
16  &  eigenvalues & Statistical & Compute the eigenvalues of covariance matrix from dataset. \\
 
17  &  g\_mean & Statistical & Compute the geometric mean of each attribute. \\
 
18  &  gravity & Statistical & Compute the distance between minority and majority classes center of mass. \\
 
19  &  h\_mean & Statistical & Compute the harmonic mean of each attribute. \\
 
20  &  iq\_rang & Statistical & Compute the interquartile range (IQR) of each attribute. \\
 
21  &  kurtosis & Statistical & Compute the kurtosis of each attribute. \\
 
22  &  lh\_trace & Statistical & Compute the Lawley-Hotelling trace. \\
 
23  &  mad & Statistical & Compute the Median Absolute Deviation (MAD) adjusted by a factor. \\
 
24  &  max & Statistical & Compute the maximum value from each attribute. \\
 
25  &  mean & Statistical & Compute the mean value of each attribute. \\
 
26  &  median & Statistical & Compute the median value from each attribute. \\
 
27  &  min & Statistical & Compute the minimum value from each attribute. \\
 
28  &  nr\_cor\_attr & Statistical & Compute the number of distinct highly correlated pairs of attributes. \\
 
29  &  nr\_disc & Statistical & Compute the number of canonical correlations between each attribute and class. \\
 
30  &  nr\_norm & Statistical & Compute the number of attributes normally distributed based in a given method. \\
 
31  &  nr\_outliers & Statistical & Compute the number of attributes with at least one outlier value. \\
 
32  &  p\_trace & Statistical & Compute the Pillai's trace. \\
 
33  &  range & Statistical & Compute the range (max-min) of each attribute. \\
 
34  &  roy\_root & Statistical & Compute the Roy's largest root. \\
 
35  &  sd & Statistical & Compute the standard deviation of each attribute. \\
 
36  &  sd\_ratio & Statistical & Compute a statistical test for homogeneity of covariances. \\
 
37  &  skewness & Statistical & Compute the skewness for each attribute. \\
 
38  &  sparsity & Statistical & Compute (possibly normalized) sparsity metric for each attribute. \\
 
39  &  t\_mean & Statistical & Compute the trimmed mean of each attribute. \\
 
40  &  var & Statistical & Compute the variance of each attribute. \\
\hline
\end{tabular}}
\end{minipage}
\end{table}

\begin{table}[H]
\centering
\begin{minipage}{0.9\linewidth}
\caption{Meta-features present in the meta-dataset}
\label{mfff}
\scalebox{0.57}{
\begin{tabular}{|l|l|l|l|}
\hline
  & Meta feature & Group & Description \\
\hline
41  &  w\_lambda & Statistical & Compute the Wilks' Lambda value. \\
 
42  &  precompute\_can\_cors & Statistical & Precompute canonical correlations and its eigenvalues. \\

43  &  precompute\_statistical\_class & Statistical & Precompute distinct classes and its abs. \\

44  &  precompute\_statistical\_cor\_cov & Statistical & Precomputes the correlation and covariance matrix of numerical data. \\

45  &  attr\_conc & Information theory & Compute concentration coef. \\

46  &  attr\_ent & Information theory & Compute Shannon's entropy for each predictive attribute. \\

47  &  class\_conc & Information theory & Compute concentration coefficient between each attribute and class. \\

48  &  class\_ent & Information theory & Compute target attribute Shannon's entropy. \\

49  &  eq\_num\_attr & Information theory & Compute the number of attributes equivalent for a predictive task. \\

50  &  joint\_ent & Information theory & Compute the joint entropy between each attribute and class. \\

51  &  mut\_inf & Information theory & Compute the mutual information between each attribute and target. \\

52  &  ns\_ratio & Information theory & Compute the noisiness of attributes. \\

53  &  precompute\_class\_freq & Information theory & Precompute each distinct class (absolute) frequencies. \\

54  &  precompute\_entropy & Information theory & Precompute various values related to Shannon's Entropy. \\

55  &  extract\_table & Model-based & Bookkeep some information table from the t\_model into an array. \\

56  &  leaves & Model-based & Compute the number of leaf nodes in the DT model. \\

57  &  leaves\_branch & Model-based & Compute the size of branches in the DT model. \\

58  &  leaves\_corrob & Model-based & Compute the leaves corroboration of the DT model. \\

59  &  leaves\_homo & Model-based & Compute the DT model Homogeneity for every leaf node. \\

60  &  leaves\_per\_class & Model-based & Compute the proportion of leaves per class in DT model. \\

61  &  nodes & Model-based & Compute the number of non-leaf nodes in DT model. \\

62  &  nodes\_per\_attr & Model-based & Compute the ratio of nodes per number of attributes in DT model. \\

63  &  nodes\_per\_inst & Model-based & Compute the ratio of non-leaf nodes per number of instances in DT model. \\

64  &  nodes\_per\_level & Model-based & Compute the ratio of number of nodes per tree level in DT model. \\

65  &  nodes\_repeated & Model-based & Compute the number of repeated nodes in DT model. \\

66  &  tree\_depth & Model-based & Compute the depth of every node in the DT model. \\

67  &  tree\_imbalance & Model-based & Compute the tree imbalance for each leaf node. \\

68  &  tree\_shape & Model-based & Compute the tree shape for every leaf node. \\

69  &  var\_importance & Model-based & Compute the features importance of the DT model for each attribute. \\

70  &  precompute\_model\_based\_class & Model-based & Precompute the DT Model and some information related to it. \\

71  &  best\_node & Landmarking & Performance of the best single decision tree node. \\

72  &  elite\_nn & Landmarking & Performance of Elite Nearest Neighbor. \\

73  &  linear\_discr & Landmarking & Performance of the Linear Discriminant classifier. \\

74  &  naive\_bayes & Landmarking & Performance of the Naive Bayes classifier. \\

75  &  one\_nn & Landmarking & Performance of the 1-Nearest Neighbor classifier. \\

76  &  random\_node & Landmarking & Performance of the single DT node model induced by a random attribute. \\

77  &  worst\_node & Landmarking & Performance of the single DT node model induced by the worst informative attribute. \\

78  &  precompute\_landmarking\_kfolds & Landmarking & Precompute k-fold cross-validation related values. \\

79  &  precompute\_landmarking\_sample & Landmarking & Precompute subsampling landmarking subsample indices. \\

80  &  group\_mtf\_by\_summary & Relative Landmarking & Group meta features by its correspondent summary method. \\

\hline
\end{tabular}}
\end{minipage}
\end{table}

\begin{table}[H]
\centering
\begin{minipage}{0.9\linewidth}
\caption{Meta-features present in the meta-dataset}
\label{mfff}
\scalebox{0.57}{
\begin{tabular}{|l|l|l|l|}
\hline
  & Meta feature & Group & Description \\
\hline
81  &  postprocess\_landmarking\_relative & Relative Landmarking & Generate Relative Landmarking from Landmarking metafeatures. \\

82  &  ch & Clustering & Compute the Calinski and Harabasz index. \\

83  &  int & Clustering & Compute the INT index. \\

84  &  nre & Clustering & Compute the normalized relative entropy. \\

85  &  pb & Clustering & Compute the Pearson correlation between class matching and instance distances. \\

86  &  sc & Clustering & Compute the number of clusters with sizes smaller than a given size. \\

87  &  sil & Clustering & Compute the mean silhouette value. \\

88  &  vdb & Clustering & Compute the Davies and Bouldin Index. \\

89  &  vdu & Clustering & Compute the Dunn Index. \\

90  &  precompute\_class\_representatives & Clustering & Precomputations related to cluster representative instances. \\

91  &  precompute\_clustering\_class & Clustering & Precompute distinct classes and its frequencies from y. \\

92  &  precompute\_group\_distances & Clustering & Precompute distance metrics between instances. \\

93  &  precompute\_nearest\_neighbors & Clustering & Precompute the n\_neighbors Nearest Neighbors of every instance. \\

94  &  cohesiveness & Concept & Improved weighted distance that captures how dense or sparse is the example distribution. \\

95  &  conceptvar & Concept & Compute the concept variation that estimates the variability of class labels among examples. \\

96  &  impconceptvar & Concept & Compute the improved concept variation that estimates the variability of class labels among examples. \\

97  &  wg\_dist & Concept & Compute the weighted distance and that captures how dense or sparse is the example distribution. \\

98  &  precompute\_concept\_dist & Concept & Precompute some useful things to support complexity measures. \\

99  &  one\_itemset & Itemset & Compute the one itemset meta-feature. \\

100  &  two\_itemset & Itemset & Compute the two itemset meta-feature. \\

101  &  precompute\_binary\_matrix & Itemset & Precompute the binary representation of attributes. \\

102  &  c1 & Complexity & Compute the entropy of class proportions. \\

103  &  c2 & Complexity & Compute the imbalance ratio. \\

104  &  cls\_coef & Complexity & Clustering coefficient. \\

105  &  density & Complexity & Average density of the network. \\

106  &  f1 & Complexity & Maximum Fisher's discriminant ratio. \\

107  &  f1v & Complexity & Directional-vector maximum Fisher's discriminant ratio. \\

108  &  f2 & Complexity & Volume of the overlapping region. \\

109  &  f3 & Complexity & Compute feature maximum individual efficiency. \\

110  &  f4 & Complexity & Compute the collective feature efficiency. \\

111  &  hubs & Complexity & Hub score. \\

112  &  l1 & Complexity & Sum of error distance by linear programming. \\

113  &  l2 & Complexity & Compute the OVO subsets error rate of a linear classifier. \\

114  &  l3 & Complexity & Non-Linearity of a linear classifier. \\

115  &  lsc & Complexity & Local set average cardinality. \\

116  &  n1 & Complexity & Compute the fraction of borderline points. \\

117  &  n2 & Complexity & Ratio of intra and extra class nearest neighbor distance. \\

118  &  n3 & Complexity & Error rate of the nearest neighbor classifier. \\

119  &  n4 & Complexity & Compute the non-linearity of the k-NN Classifier. \\

120  &  t1 & Complexity & Fraction of hyperspheres covering data. \\

\hline
\end{tabular}}
\end{minipage}
\end{table}

\begin{table}[H]
\centering
\begin{minipage}{0.9\linewidth}
\caption{Meta-features present in the meta-dataset}
\label{mfff}
\scalebox{0.7}{
\begin{tabular}{|l|l|l|l|}
\hline
  & Meta feature & Group & Description \\
\hline
121  &  t2 & Complexity & Compute the average number of features per dimension. \\

122  &  t3 & Complexity & Compute the average number of PCA dimensions per point. \\

123  &  t4 & Complexity & Compute the ratio of the PCA dimension to the original dimension. \\

124  &  precompute\_adjacency\_graph & Complexity & Calculate values associated with the nearest neighboring instances. \\

125  &  precompute\_complexity & Complexity & Precompute some useful things to support feature-based measures. \\

126  &  precompute\_complexity\_svm & Complexity & Init a Support Vector Classifier pipeline (with data standardization.) \\

127  &  precompute\_nearest\_enemy & Complexity & Precompute instances nearest enemy related values. \\

128  &  precompute\_norm\_dist\_mat & Complexity & Precompute normalized n and pairwise distance among instances. \\

129  &  precompute\_pca\_tx & Complexity & Precompute PCA to support dimensionality measures. \\

\hline
\end{tabular}}
\end{minipage}
\end{table}
